# Supplementary material for: DVMNet++: Rethinking Relative Pose Estimation for Unseen Objects
Source: arXiv:2403.13683 source file (2025-03-15)
Supplement: Supplementary file 1 [file X_suppl.tex]

\clearpage
\setcounter{page}{1}

\section*{6D Relative Object Pose Estimation}
\label{sec:6d}
As introduced in the main paper, we are interested in extending the presented DVMNet to 6D relative object pose estimation in our future work. Notably, we followed the setting proposed in RelPose, RelPose++, and 3DAHV, assuming the availability of known object positions. Such information provides a strong prior, making the relation translation estimation less challenging. In this scenario, the primary challenge is the detection of an unseen object present in the query image. We achieve the zero-shot object detection by utilizing the detection module presented in Gen6D~\cite{liu2022gen6d}. Specifically, the detection module predicts the 2D object center and 2D object scale, from which we compute the 3D object translation, following the implementation of Gen6D. The 3D object rotation is estimated by employing our DVMNet. It is worth noting that our goal is to achieve 6D object pose estimation in the single-reference setup, while Gen6D's detection module utilizes dense-view references by default. Therefore, in our experiments, we feed a single reference to the detection module as the template. 

We illustrate some preliminary results in Fig.~\ref{fig:viz_6d} and Fig.~\ref{fig:viz_6d_fail}, visualizing the 6D object pose in the query image as a 3D object bounding box. As shown in Fig.~\ref{fig:viz_6d}, the combination of Gen6D's object detector and our DVMNet achieves promising results in some cases. However, in some scenarios shown in Fig.~\ref{fig:viz_6d_fail}, Gen6D's detector fails to effectively detect the unseen object depicted in the query image. Notably, the zero-shot object detection becomes more challenging in the single-reference setting due to the large pose difference between the query object and the reference. In this context, we plan to investigate the applicability of other zero-shot object detectors such as SAM~\cite{kirillov2023segment} in future work.

\begin{figure}[!t]
    \centering	
    \includegraphics[width=1.0\linewidth]{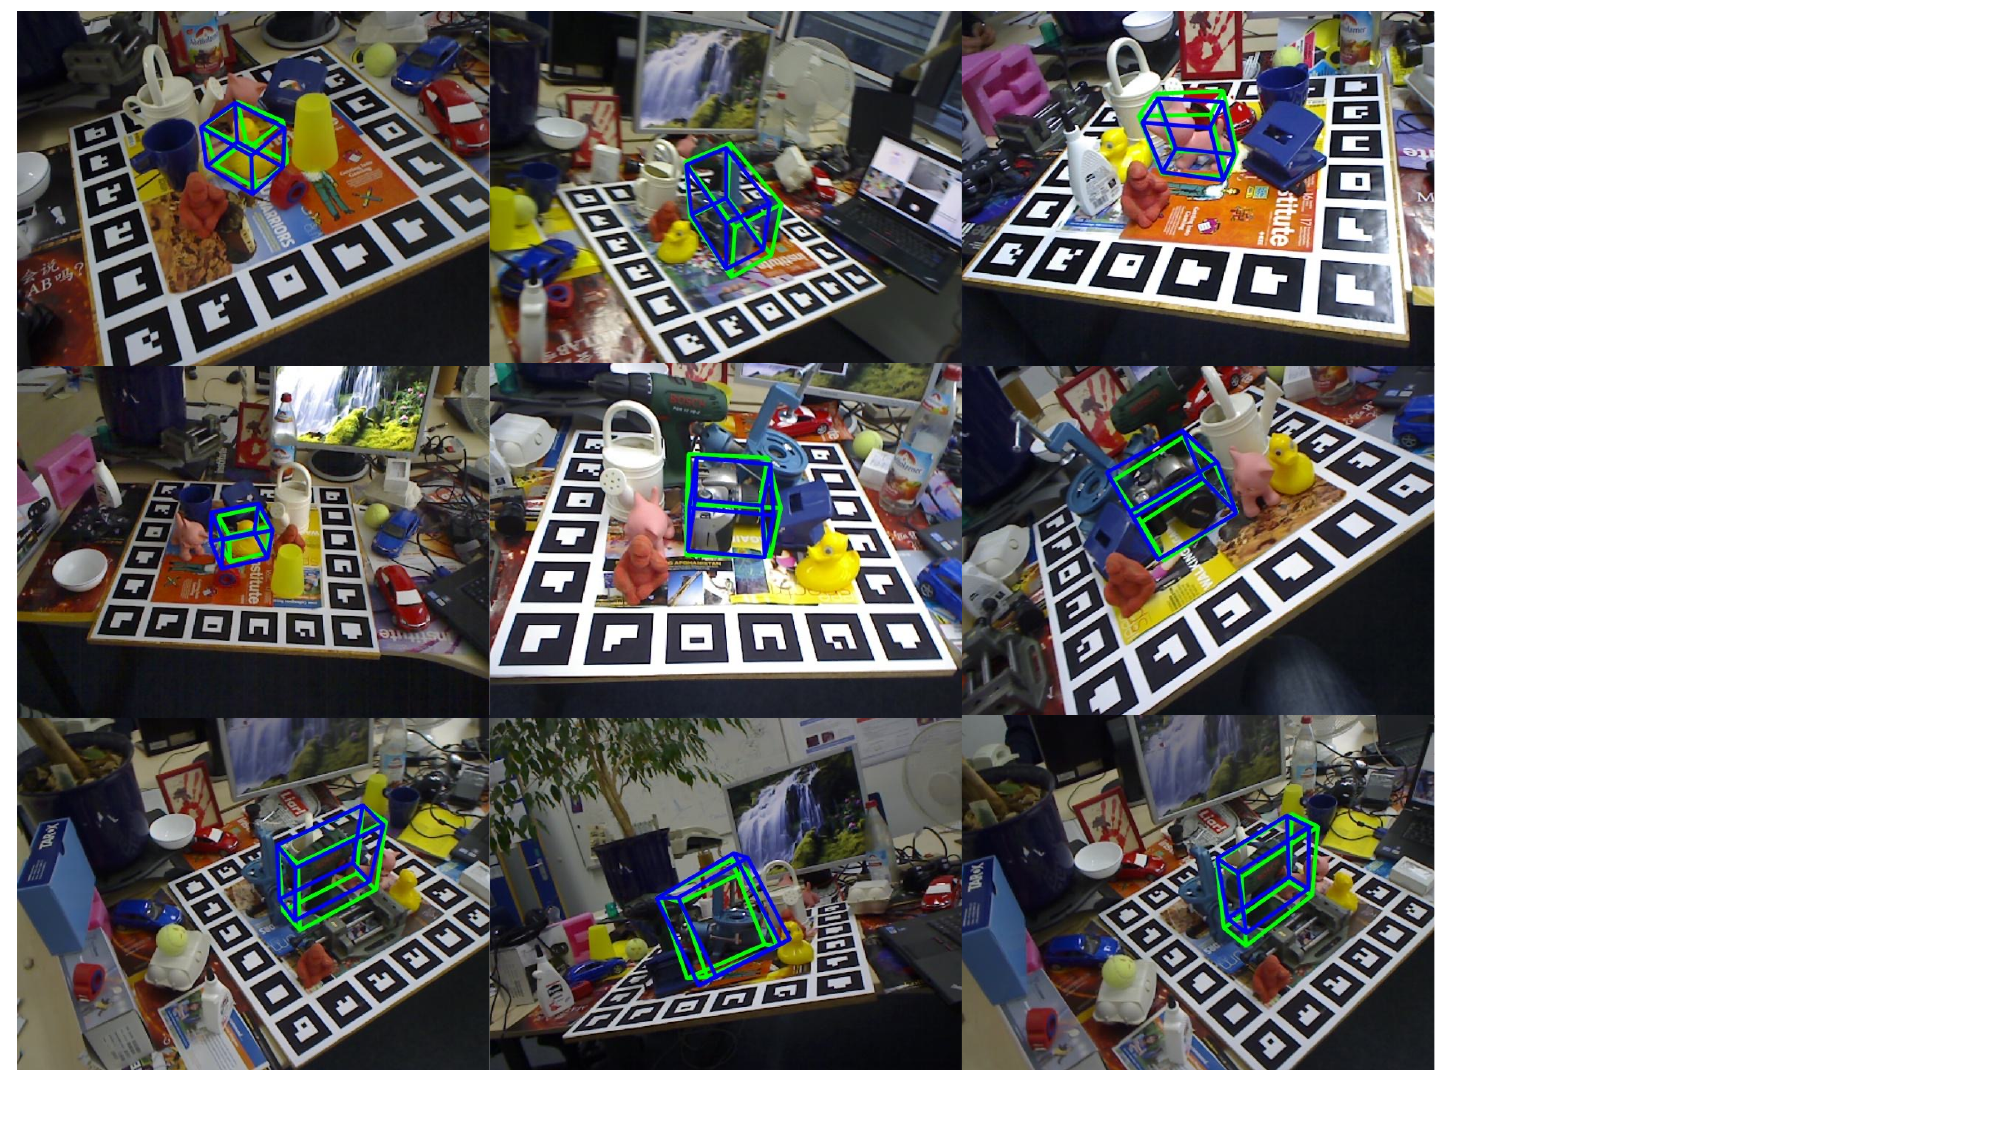}
    \caption{\textbf{Visualization of 6D pose estimation for unseen objects on LINEMOD~\cite{hinterstoisser2012model}.} The ground-truth 6D object pose and the predicted pose in the query image are depicted as green and blue 3D bounding boxes, respectively.}
    \label{fig:viz_6d}
\end{figure}

\begin{figure}[!t]
    \centering	
    \includegraphics[width=1.0\linewidth]{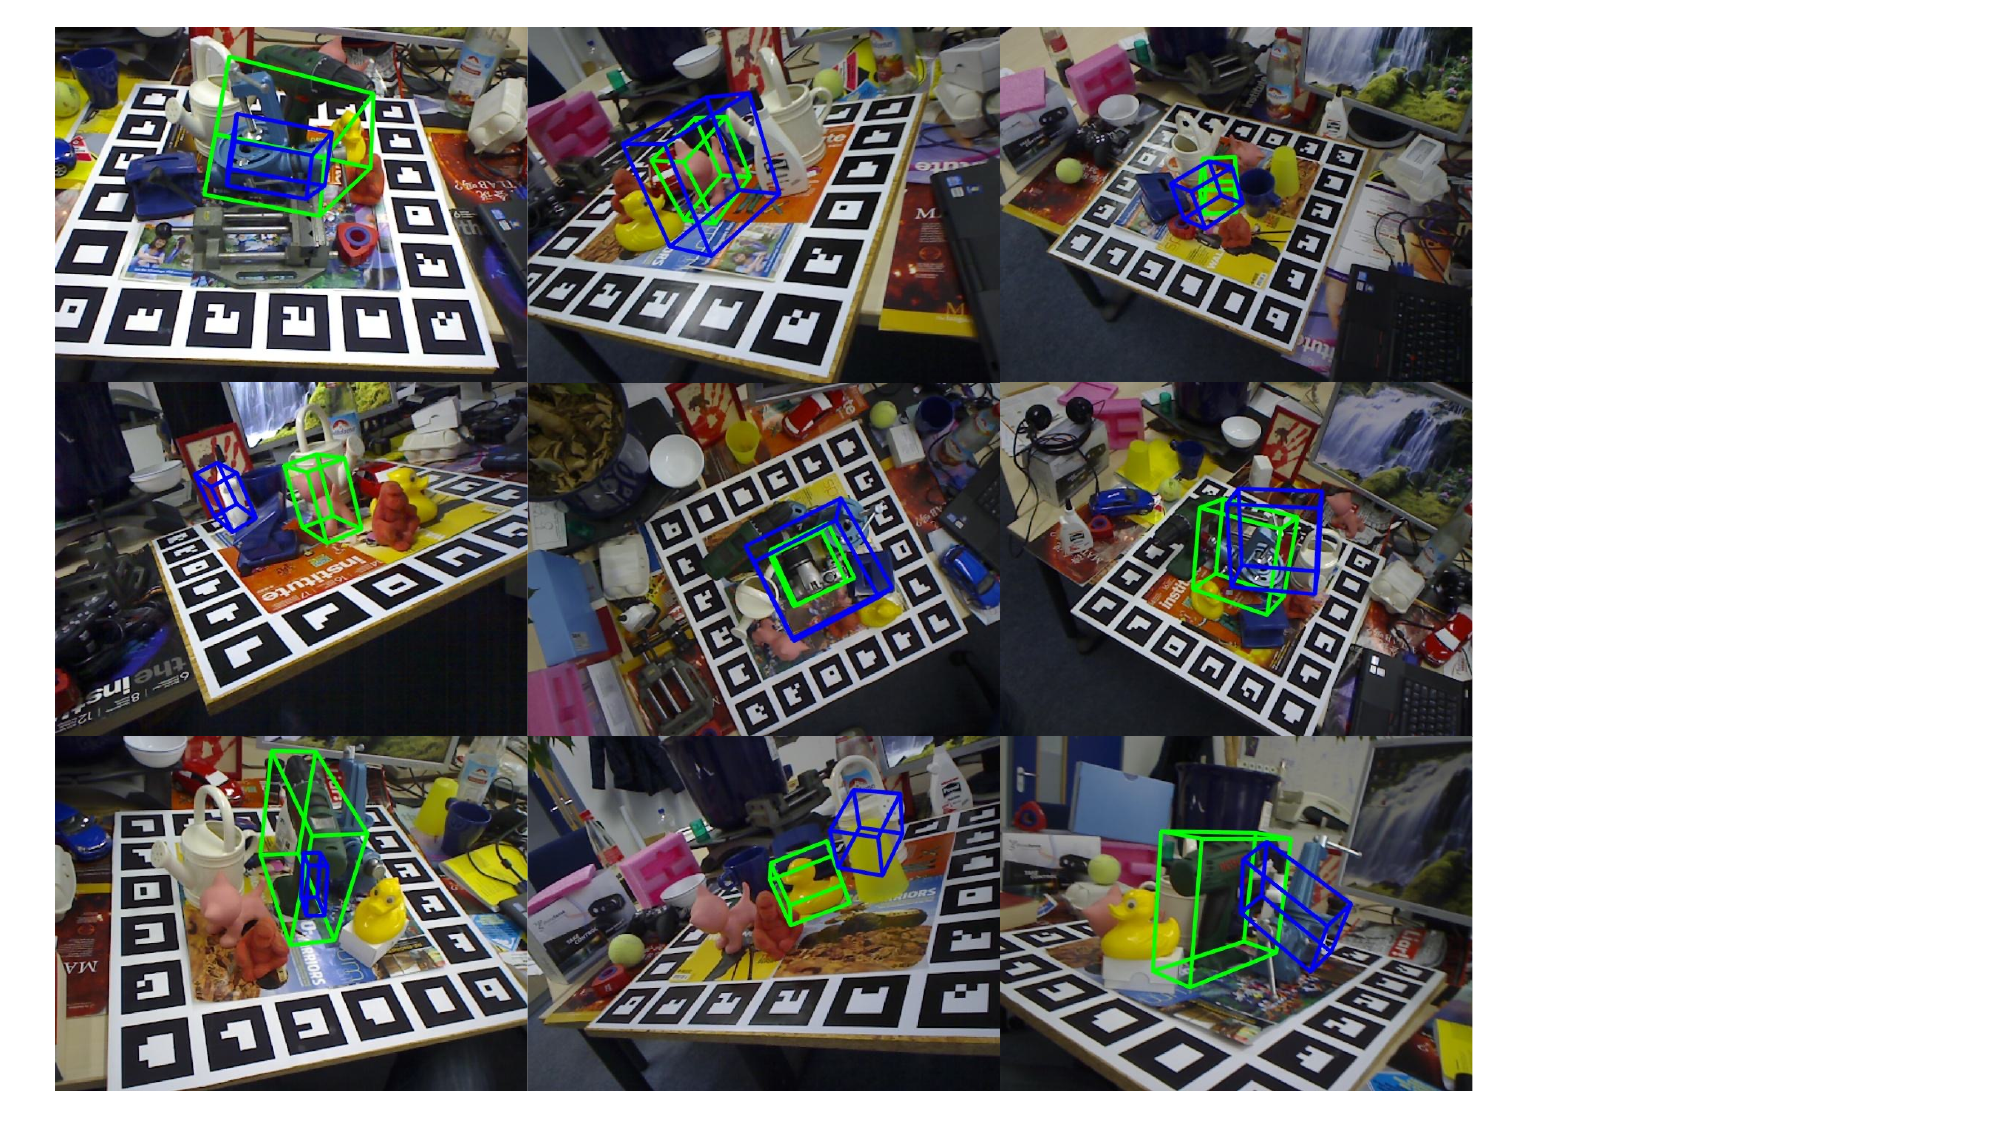}
    \caption{\textbf{Failure cases of 6D pose estimation for unseen objects on LINEMOD~\cite{hinterstoisser2012model}.} }
    \label{fig:viz_6d_fail}
\end{figure}

\section*{Extension to Sparse-View References}
\label{sec:sparse}

\begin{table*}[!t]
    \centering
    \begin{tabular}{lccccccc}
    \Xhline{2\arrayrulewidth}
    \# References & 1     & 2     & 3     & 4     & 5     & 6     & 7     \\
    \hline
    SuperGlue & 71.47 & 73.08 & 68.72 & 65.90 & 64.54 & 63.24 & 61.74 \\
    3DAHV & 28.44 & 29.29 & 28.20 & 27.21 & 26.40 & 24.85 & 24.76 \\
    DVMNet & \textbf{19.95} & \textbf{18.38} & \textbf{16.79} & \textbf{16.21} & \textbf{15.73} & \textbf{14.99} & \textbf{14.93} \\
    \Xhline{2\arrayrulewidth}
    \end{tabular}
    \caption{\textbf{Extension to sparse-view references.} The experiment is conducted on CO3D~\cite{reizenstein2021common} with the number of reference images varying from 1 to 7. The metric employed is the angular error between the computed query object pose and the ground truth.}
    \label{tab:sparse}
\end{table*}

As introduced in the literature~\cite{schonberger2016structure,zhang2022relpose,lin2023relpose++}, some downstream tasks such as 3D reconstruction often rely on sparse-view references. Intuitively, our DVMNet can be seamlessly integrated into these tasks, as it operates effectively with just a single reference. Therefore, we develop an experiment on the CO3D dataset, evaluating DVMNet with varying numbers of reference images, ranging from 1 to 7. 

Specifically, given an unseen object during testing, we randomly sample $n$ images. These images are then fed into the presented DVMNet, with one image designated as the query and the remaining ones as references. The object pose in the query image is simply derived from the resulting $n-1$ relative object poses as
\begin{align}
\label{eq:sparse}
\mathbf{R}_q=m(\frac{1}{n-1}\sum_{i=1}^{n-1}q(\Delta\mathbf{R}_i \mathbf{R}_r^{i})),
\end{align}
where $\Delta\mathbf{R}_i$ and $\mathbf{R}_r^{i}$ denote the $i$-th relative object pose and reference pose, respectively, $q(\cdot)$ represents a function that converts a rotation matrix to the 6D continuous representation~\cite{zhou2019continuity}, and $m(\cdot)$ indicates the conversion from the 6D continuous representation to a rotation matrix. We also evaluate the representative image-matching (SuperGlue) and hypothesis-based (3DAHV) approaches in the sparse-view scenario. We ensure a fair comparison by utilizing the same strategy of query object pose estimation for these methods.

We report the resulting angular errors in Table~\ref{tab:sparse}. It is evident that (i) the angular error of our DVMNet decreases as more reference images are involved, and (ii) DVMNet consistently yields the smallest angular error. This observation demonstrates the promising compatibility of our approach with sparse-view reference images.

\section*{Robustness to Occlusions}
\label{sec:occ}
\begin{table}[!t]
    \centering
    \begin{tabular}{lccc}
    \Xhline{2\arrayrulewidth}
    Method        & SuperGlue & 3DAHV & DVMNet \\
    \hline
    Angular Error $\downarrow$ & 73.72 & 51.49 & 49.02 \\
    \Xhline{2\arrayrulewidth}
    \end{tabular}
    \caption{\textbf{Experimental results on the LINEMOD-O~\cite{brachmann2014learning} dataset.} The mean angular errors are reported.}
    \label{tab:lmo}
\end{table}
Given that object pose estimation is often challenged by occlusions, we assess the robustness in scenarios involving occlusions by conducting an experiment on the LINEMOD-O~\cite{brachmann2014learning} dataset. The testing data comprises three unseen objects, i.e., cat, driller, and duck. We report the mean angular errors of the evaluated methods in Table~\ref{tab:lmo}. Our DVMNet outperforms both the image-matching method, SuperGlue, and the hypothesis-based method, 3DAHV, showcasing better robustness against occlusions.

\begin{table}[!t]
    \begin{center}
        \begin{tabular}{lcc}
        \Xhline{2\arrayrulewidth}
        Method &  Acc @ $30^{\circ}$ (\%) $\uparrow$ \\
        \hline
        RelPose & 64.2 \\
        RelPose++ & 77.0 \\
        3DAHV & 83.5 \\
        PoseDiffusion & 81.8 \\
        DVMNet & \textbf{84.7} \\
        \hline 
        \Xhline{2\arrayrulewidth}
        \end{tabular}
    \end{center}
    \caption{\textbf{Additional experimental results on CO3D.} Acc @ $30^{\circ}$ is employed as a metric.}
    \label{tab:co3d_acc30}
\end{table}

\section*{Additional Results on CO3D}
\label{sec:add}
As listed in Tabel~\ref{tab:co3d_acc30}, we report more results on CO3D, using Acc @ $30^{\circ}$ as a metric. Note that PoseDiffusion~\cite{wang2023posediffusion} takes multiple views ($>2$) as input by default, while all the other evaluated methods employ two views. For a fair comparison, we evaluate PoseDiffusion on CO3D using two views. Moreover, The pose parameters are iteratively updated 100 times during the denoising process in PoseDiffusion, making the method time-consuming compared with our single forward pass mechanism.

\clearpage
